# Supplementary material for: Improving the Behaviour of Vision Transformers with Token-consistent Stochastic Layers
Source: arXiv:2112.15111 source file (2022-07-14)
Supplement: Supplementary file 1 [file adv_robustness.tex]

\begin{table}[t!]
\centering
\tableFont
\captionsetup{font=small}
\caption{{\textbf{Adversarial robustness, with adversarial training.} Our stochastic layers increase adversarial robustness in vision transformers. Combining the effects of strong noise with monte-carlo sampling can improve adversarial robustness and clean accuracy under adversarial training.}}
%\resizebox{\columnwidth}{!}{
%\renewcommand\arraystretch{1}
%\resizebox{\columnwidth}{!}{
%\centering
\begin{tabular}{|l|l||c|c||c|c|}
\hline

\multicolumn{6}{|c|}{\makecell{Accuracy $\uparrow$}} \\ \hline

%\multicolumn{3}{|c|}{} & \multicolumn{3}{|c|}{\makecell{Without adversarial training}} \\ \cline{4-6}
  
\multicolumn{2}{|c||}{} 
 %& Clean
 & \multicolumn{2}{|c||}{\makecell{Adversarial training \\ with $\epsilon=2$}} 
 & \multicolumn{2}{|c|}{\makecell{Adversarial training \\ with $\epsilon=4$}}
 \\ \cline{3-6}
 
\multicolumn{2}{|c||}{} 
 & \makecell{Clean \\ samples}
 & {\makecell{PDG$-10$ \\ attack}} 
 & \makecell{Clean \\ samples}
 & {\makecell{PDG$-10$ \\ attack}}
 \\ \hline \hline 
 
\multicolumn{2}{|c||}{Regular} & $71.61\%$ & $42.33\%$ & $65.04\%$ & $27.24\%$  \\ \hline 

% \multirow{6}{*}{\makecell{ Training \\ $\Delta=0.1$}}
%  & Ours $N=1$  & $71.79\%$ & $42.90\%$ & $65.23\%$ & $27.88\%$ \\ \cline{2-6} 
%  & Ours $N=50$ & $71.84\%$ & $42.91\%$ & $65.29\%$ & $27.86\%$ \\ \cline{2-6}
%  & Uniform everywhere $N=1$  & $\%$ & $\%$ & $\%$ & $\%$ \\ \cline{2-6} 
%  & Uniform everywhere $N=50$  & $\%$ & $\%$ & $\%$ & $\%$ \\ \cline{2-6} 
%  & Dropout $N=1$  & $\%$ & $\%$ & $\%$ & $\%$ \\ \cline{2-6} 
%  & Dropout $N=50$  & $\%$ & $\%$ & $\%$ & $\%$ \\ \hline 

\multirow{6}{*}{\makecell{ Training \\ $\Delta=0.5$}}
 &DeiT-S ($N=1)$& $71.79\%$ & $44.51\%$ & $66.53\%$ & $30.68\%$ \\ \cline{2-6} 
 &DeiT-S ($N=50)$& $73.73\%$ & $46.21\%$ & $68.65\%$ & $31.47\%$ \\ \cline{2-6} 
 &DeiT-S + non-token-consistent ($N=1)$& $73.64\%$ & $45.89\%$ & $69.27\%$ & $32.25\%$ \\ \cline{2-6} 
 &DeiT-S + non-token-consistent ($N=50)$& $74.60\%$ & $46.49\%$ & $70.25\%$ & $32.62\%$ \\ \cline{2-6} 
 &DeiT-S + dropout ($N=1)$& $73.39\%$ & $45.77\%$ & $68.87\%$ & $32.02\%$ \\ \cline{2-6} 
 &DeiT-S + dropout ($N=50)$& $74.47\%$ & $46.44\%$ & $70.07\%$ & $32.44\%$ \\ \hline 
 
\multirow{6}{*}{\makecell{ Training \\ $\Delta=1.0$}}
 &DeiT-S ($N=1)$& $68.62\%$ & $45.37\%$ & $65.40\%$ & $33.48\%$  \\ \cline{2-6}  
 &DeiT-S ($N=50)$& $73.83\%$ & $49.32\%$ & $70.47\%$ & $36.38\%$  \\ \cline{2-6}
 &DeiT-S + non-token-consistent ($N=1)$& $72.87\%$ & $48.79\%$ & $69.88\%$ & $36.98\%$ \\ \cline{2-6}
 &DeiT-S + non-token-consistent ($N=50)$& $75.23\%$ & $50.75\%$ & $72.35\%$ & $38.03\%$ \\ \cline{2-6} 
 &DeiT-S + dropout ($N=1)$& $73.11\%$ & $48.68\%$ & $69.95\%$ & $36.96\%$ \\ \cline{2-6} 
 &DeiT-S + dropout ($N=50)$& $75.28\%$ & $50.58\%$ & $72.24\%$ & $38.00\%$ \\ \hline 
\end{tabular}
%}

\label{table:supp_adv_robustness}
\end{table}
