# Supplementary material for: Improving the Behaviour of Vision Transformers with Token-consistent Stochastic Layers
Source: arXiv:2112.15111 source file (2022-07-14)
Supplement: Supplementary file 2 [file calibration_no_temperature.tex]

\begin{table}[t!]
\centering
\tableFont
\captionsetup{font=small}
\caption{{\textbf{Confidence calibration without temperature tuning}. We observe that the confience calibration is much worse without using temperature tuning. For results with temperature tunin, please take a look at Table~\ref{table:supp_calibration_with_temp}}.}
%\begin{adjustbox}{\columnwidth}
%\renewcommand\arraystretch{1}
\begin{tabular}{|l|l|c|c|c|}
\hline
\multicolumn{2}{|c|}{} & \multicolumn{3}{c|}{ECE$\downarrow$}  \\ \cline{3-5}
\multicolumn{2}{|c|}{} & $\Delta=0$  & $N=1$ & $N=50$         \\ \hline \hline

\multicolumn{2}{|l|}{Regular} & $0.087$ & $0.087$ & $0.087$  \\ \hline \hline

\multirow{2}{*}{\makecell{Training \\ $\Delta=0.5$}} 
 & Dropout         & $0.087$ & $0.091$ & $0.083$ \\ \cline{2-5}
 & Ours  & $0.090$ & $0.101$ & $0.112$ \\ \hline \hline
 
\multirow{2}{*}{\makecell{Training \\ $\Delta=1.0$}} 
 & Dropout         & $0.092$ & $0.102$ & $0.103$ \\ \cline{2-5}
 & Ours  & $0.092$ & $0.104$ & $0.130$ \\ \hline

\end{tabular}
\label{table:supp_calibration_no_temp}
\end{table}
